# Supplementary material for: A Ubiquitous Thermal Conductivity Formula for Liquids, Polymer Glass, and Amorphous Solids
Source: arXiv:2005.00217 source file (2020-09-26)
Supplement: Supplementary file 1 [file Supplementary.pdf]

# Supplementary Information for "A ubiquitous thermal conductivity formula for liquids, polymer glass and amorphous solids"

Qing Xi,[1] Jinxin Zhong,[1] Jixiong He,[2] Xiangfan Xu,[1] Tsuneyoshi Nakayama,[1,3] Yuanyuan Wang,[4] Jun Liu,[2,*] Jun Zhou,[1,†] and Baowen Li[5,‡]

[1]*Center for Phononics and Thermal Energy Science, China-EU Joint Lab for Nanophononics, School of Physics Science and Engineering, Tongji University, Shanghai 200092, China*

[2]*Department of Mechanical and Aerospace Engineering, North Carolina State University, Raleigh, NC 27695, USA*

[3]*Hokkaido University, Sapporo, Hokkaido 060-0826, Japan*

[4]*School of Environmental and Materials Engineering, Shanghai Polytechnic University, Shanghai 201209, China*

[5]*Paul M Rady Department of Mechanical Engineering, Department of Physics, University of Colorado, Boulder, CO 80305-0427, USA*

(Dated: September 19, 2020)

## SA. Fundamental units transferring heat in molecular liquids and amorphous molecular solids

In liquids and amorphous solids made of weakly coupled molecules, the fundamental units characterizing thermal conduction are individual molecules, whose atomic arrangement can be described by relatively close packing with voids in liquids and random packing in solid.

### *Molecular Liquids*

The kinetic theory of gases (KTG) fails to explain the thermal transport in liquids because the molecules are neither localized around fixed equilibrium positions like in solids nor move freely like gases. Tranchenko and Brazhkin [1] have demonstrated that the thermodynamical properties of simple liquids are determined by the vibrational contributions as in solids in all range of liquid relaxation times [2, 3]. In other words, the characteristic time of thermal transport is shorter than the duration between two events of jump of certain atom accompanied by large scale rearrangement of its surrounding atoms. The surrounding atoms can be seen as temporary touching neighbours. We have evaluated the coordination number of touching neighbours for several typical liquids by the Monte Carlo simulation. The simulation details are given in section SD and the results are shown in Table S1.

Using the simulated $Z$, we further calculated the thermal conductivities by Eq. (1) with $\tilde{n} = \rho/m_{\mathrm{mole}}$, $\Xi = 2$, and $\gamma = 1$, and it is reduced to Eq. (3) with $\alpha = \left(\frac{Z}{6}\frac{\rho}{m_{\mathrm{mole}}}\right)^{\frac{1}{3}}$. $\delta = a$ should be used for most molecules, where $a$ is the Van der Waals diameter of molecule. The only exception is benzene because of its ring structure. The calculated thermal conductivities using parameters in Table. S1 are shown in Fig. 2(a) and (b) in comparison with the experimentally measured data. Figure 2(a) gives the thermal conductivities of various liquids, whose aspect ratio is $L/a < 2$, including methanol, carbon tetrachloride, benzene, chloroform, water, acetic acid, acetone, carbon disulfide, butyl alcohol, butyric acid, glycerol, N-propanal, and isopropanol. The calculated values are in excellent agreement with the experimental values by choosing $D_v$ to be 1∼3 for nearly spherical molecules ($L/a \sim 1$) and $D_v = 1$ for non-spherical molecules ($L/a > 1$). For alkanes whose aspect ratio is $L/a > 2$, we find that the calculated thermal conductivities perfectly match the experimental values by choosing $D_v = 1$ as shown in Fig. 2(b). The reduction of $D_v$ for liquids with long molecules originates from the higher possibility of thermal transport along the longitudinal axis of molecules while it is hard to transport along the transverse axis. This feature can be understood as an analogy of reptation of molecules [4].

We now revisit the Bridgman's formula. In his original paper, Bridgman considered six nearest neighbours forming a simple lattice structure. Adopting this structure, it is easy to reproduce the Bridgman's formula from Eq. (3) by taking $Z = 6$, $\gamma = 1$, $D_v = 3$, $\tilde{n} = n_{\mathrm{mole}}$, and $\delta = n_{\mathrm{mole}}^{-\frac{1}{3}}$. We shall point out that the Bridgman's formula is applicable only when the molecules are nearly-spherical. For nearly-spherical molecules (such as methanol, carbon tetrachloride, chloroform, and water), the calculated values of $Z$ are between 4.4∼5.3 as shown in Table. S1. This results in 0.90< $\left(\frac{Z}{6}\right)^{\frac{1}{3}}$ <0.96. We further compare $a$ with $n_{\mathrm{mole}}^{-\frac{1}{3}}$ by taking methanol and carbon tetrachloride as examples. We find that the values $n_{\mathrm{mole}}^{-\frac{1}{3}} = 4.07$Å for methanol and 5.43Å for carbon tetrachloride are very close to their diameters 4.2Å and 5.6Å, respectively. Therefore, $a \approx n_{\mathrm{mole}}^{-\frac{1}{3}}$ is valid in liquids with nearly spherical molecules.

The Bridgman's formula breaks down for non-spherical molecules. This discrepancy comes from the enhancement of $Z$ with increasing $L$ and the significant difference between $a$ and $n_{\mathrm{mole}}^{-\frac{1}{3}}$. For example, $n_{\mathrm{mole}}^{-\frac{1}{3}} = 7.88$Å for $C_{16}H_{34}$ is much larger than its diameter 4Å. We further compare the thermal conductivities between isomers by taking N-propanal and isopropanol as an example. They have exactly the same chemical composition, $C_3H_7OH$. The observed thermal conductivities of N-propanal and isopropanol are 0.155 $\mathrm{Wm^{-1}K^{-1}}$ and 0.137 $\mathrm{Wm^{-1}K^{-1}}$, respectively. Their relative difference is 13%. The calculated results from our formula Eq. (1) are 0.150 $\mathrm{Wm^{-1}K^{-1}}$ and 0.131 $\mathrm{Wm^{-1}K^{-1}}$ by taking $D_v = 1$.

TABLE S1. Mass density, molecular length, molecular diameter, molar mass, and sound velocity of typical liquids used in the calculations [5, 6]. $Z$ is calculated by Monte Carlo simulation except for water which is taken from Ref. [7].

| Liquids | $\rho$ (g/cm$^3$) | $L$ (Å) | $a$ (Å) | $M_{\rm mole}$ (g/mol) | $v_s$ (m/s) | $Z$ |
|---|---|---|---|---|---|---|
| Methanol ($CH_3OH$) | 0.787 | - | 4.2 | 32.04 | 1076 | 4.59 |
| Carbon tetrachloride ($CCl_4$) | 1.594 | - | 5.6 | 153.8 | 926 | 4.59 |
| Benzene ($C_6H_6$) | 0.876 | - | 5.4 | 78.11 | 1321 | 4.45 |
| Chloroform ($CHCl_3$) | 1.479 | - | 5.2 | 119.37 | 979 | 4.40 |
| Water ($H_2O$) | 0.998 | - | 2.8 | 18.015 | 1482 | 4.7,5.3 |
| Acetic acid ($CH_3COOH$) | 1.045 | 4.99 | 4.0 | 60.05 | 1150 | 4.03 |
| Acetone ($CH_3COCH_3$) | 0.784 | 6.54 | 4.0 | 58.08 | 1190 | 4.84 |
| Carbon disulfide ($CS_2$) | 1.263 | 4.94 | 4.0 | 76.15 | 1158 | 3.26 |
| Butyl alcohol ($C_4H_{10}O$) | 0.810 | 7.26 | 4.0 | 74.12 | 1222 | 4.62 |
| Butyric acid ($C_4H_8O_2$) | 0.959 | 7.26 | 4.0 | 88.11 | 1380 | 4.63 |
| Glycerol ($C_3H_8O_3$) | 1.261 | 6.71 | 4.0 | 92.09 | 1920 | 5.13 |
| N-propanol ($C_3H_7OH$) | 0.805 | 5.99 | 4.0 | 60.1 | 1220 | 4.20 |
| isopropanol ($C_3H_7OH$) | 0.785 | 5.27 | 4.0 | 60.1 | 1170 | 3.27 |
| $C_6H_{14}$ | 0.659 | 10.35 | 4.0 | 86.18 | 1113 | 5.85 |
| $C_7H_{16}$ | 0.680 | 11.62 | 4.0 | 100.2 | 1131 | 6.33 |
| $C_8H_{18}$ | 0.699 | 12.89 | 4.0 | 114.23 | 1213 | 6.78 |
| $C_9H_{20}$ | 0.718 | 14.16 | 4.0 | 128.25 | 1226 | 7.33 |
| $C_{10}H_{22}$ | 0.726 | 15.43 | 4.0 | 142.28 | 1252 | 7.75 |
| $C_{12}H_{26}$ | 0.750 | 17.97 | 4.0 | 170.33 | 1279 | 8.74 |
| $C_{13}H_{28}$ | 0.756 | 19.24 | 4.0 | 184.36 | 1278 | 9.19 |
| $C_{14}H_{30}$ | 0.763 | 20.51 | 4.0 | 198.39 | 1294 | 9.68 |
| $C_{15}H_{32}$ | 0.768 | 21.78 | 4.0 | 212.41 | 1307 | 10.16 |
| $C_{16}H_{34}$ | 0.770 | 23.05 | 4.0 | 226.44 | 1338 | 10.54 |

The relative difference from our calculation is also 13% which is in excellent agreement with experimental data. The main difference comes from the decrease of the value of $Z$ as shown in Table. S1. In contrast, the Bridgman's formula gives larger values of 0.203 $\mathrm{Wm^{-1}K^{-1}}$ and 0.192 $\mathrm{Wm^{-1}K^{-1}}$. The relative difference is only 5.7%. Therefore, our formula Eq. (1) captures well the underlying chemical structural effect on thermal transport in liquids.

*Molecular amorphous Solids*

The thermal conductivity of amorphous solids composed of small molecules are considered in a similar way as liquids. In contrast to liquids, the molecules in solids vibrate at equilibrium positions and the neighbouring molecules are fixed. Then the thermal conductivity is evaluated by Eq. (3) with $\alpha = \left(\frac{Z}{6}\frac{\rho}{m_{\rm mole}}\right)^{\frac{1}{3}}$, which is close to the case of molecular liquids. The only difference is to replace $v_s$ by $\bar{v}_s$ because there are additional two transverse modes in solids.

TABLE S2. Mass density, molar mass of molecule, diameter of atom, and sound velocity of three molecular amorphous solids used in the calculations [9]. Calculated $Z$ of paraffin is shown. The values of $Z$ of a-Se and a-$As_2S_3$ are unknown because of their irregular structures.

| Molecular amorphous solids | $\rho$ (g/cm$^3$) | $M_{\rm mole}$ (g/mol) | $a$ (Å) | $v_{sl}$ (m/s) | $v_{st}$ (m/s) | $Z$ |
|---|---|---|---|---|---|---|
| Paraffin ($C_{18}H_{38}$) | 0.777 | 254.5 | 4.0 | 1400 | - | 11.43 |
| a-Se ($Se_8$ ring) | 4.30 | 631.7 | 3.80 | 2060 | 1060 | - |
| a-$As_2S_3$ | 3.20 | 246.05 | 3.60∼3.70 | 2650 | 1440 | - |

We consider paraffin, amorphous octaselenium (a-Se), and amorphous $As_2S_3$ (a-$As_2S_3$) as examples where their parameters are given in Table. S2. It has been experimentally confirmed, e.g., from the optical spectroscopy measurements, that a-Se are composed of polymeric chains and crown ring $Se_8$ molecules[10]. Since it is difficult to control this ratio in sample preparations of a-Se, we estimate $\kappa$ for two extreme cases for a-Se, one is composed of 100% of $Se_8$ molecules (in this section) and the other is 100% polymeric chains (in section SC). The calculated results for these extreme cases are given in Fig. 2 (c) and (d). We see that there exists discrepancy with the observed data of $\kappa$. This is due to that it is difficult to prepare the actual samples of two extreme cases, in addition to the difficulty to identify the detailed microscopic structures in a-Se.

Paraffin is long molecule whose $Z$ is calculated to be 11.43. The molecular structures of a-Se, which takes crown-shaped disk-like structure, and a-$As_2S_3$ are too irregular to calculate their value of $Z$ by our simple Monte Carlo simulations. Therefore, we show the results for $5 < Z < 7$ which is a typical range due to random close packing model [8]. Fig. 2(c) shows that the calculated thermal conductivities in comparison with experimental data when $D_v = 1$. The calculated thermal conductivity of a-Se (a-$As_2S_3$) is 0.152-0.170 (0.257-0.296) $\mathrm{Wm^{-1}K^{-1}}$ which is close to the experimental data 0.140 $\mathrm{Wm^{-1}K^{-1}}$ (0.246 $\mathrm{Wm^{-1}K^{-1}}$). As for comparison, the minimum thermal conductivity (MTC) formula gives an overestimated value of 0.230 $\mathrm{Wm^{-1}K^{-1}}$ (0.345$\mathrm{Wm^{-1}K^{-1}}$). Therefore, we should conclude that the MTC formula is inappropriate to calculate the thermal conductivity of molecular amorphous solids, while our formula gives the correct value.

**SB. Fundamental units in covalent-bonded amorphous solids**

In amorphous solids such as amorphous Si (a-Si), amorphous Ge (a-Ge), amorphous $CdGeAs_2$ (a-$CdGeAs_2$), and vitreous silica (v-$SiO_2$) in which atoms are covalently bonded. We should stress that atomic clusters with local order should be chosen as fundamental units. In order to reach thermal equilibrium, it should take shorter time than the heat transfer between neighbouring clusters. Such ordered clusters have been experimentally observed through radial distribution

TABLE S3. Mass density, average molar mass of atom, bond length, diameter of cluster, and sound velocity of four amorphous covalently bonded solids used in the calculations [9].

| Covalently bonded amorphous solids | $\rho$ (g/cm$^3$) | $M_{\text{atom}}$ (g/mol) | $b$ (Å) | $\zeta$ | $v_{sl}$ (m/s) | $v_{st}$ (m/s) |
|---|---|---|---|---|---|---|
| a-Si | 2.33 | 28.09 | 2.33 | 4b | 7360 | 4370 |
| a-Ge | 5.32 | 72.64 | 2.41 | 4b | 4350 | 2630 |
| v-$SiO_2$ | 2.21 | 20.03 | 1.63 | 7Å | 5980 | 3740 |
| a-$CdGeAs_2$ | 5.72 | 83.72 | 2.50 | 4b | 3030 | 1860 |

function (RDF) by X-ray diffraction where the RDF shows sharp peaks when the distance from a center atom is smaller than $2b$, where $b$ is the length of the covalent bond. We assume that the average size of fundamental units is approximately $4b$. This is consistent with the observed size of crystalline domain, for example, 7 Å for amorphous silica [11].

We assume that the amorphous solids are formed by random close packing of spherical clusters, whose volume is $V_{cl} = \frac{4\pi}{3}(\frac{\zeta}{2})^3$ where $\zeta$ is the diameter of cluster. According to the theory of random close packing, the average coordination number $Z = 6.91$ [8] and the filling factor $V_{cl}\tilde{n} = 0.637$ [12]. Therefore, the thermal conductivity can be evaluated by choosing $\Xi = 2$ and $\gamma = 1$, which leads to Eq. (3) with $\alpha = \left(\frac{6.91}{6}\frac{0.637}{V_{cl}}\right)^{\frac{1}{3}}$. If we rewrite the mass density of solid as $\frac{N_{cl}}{V_{cl}}m_{\text{atom}} = \rho$ where $N_{cl}$ is the number of atoms in each cluster. The numerical simulations showed that $N_{cl} = 14.2 + 1$ [13] which means 1 atom with 14.2 neighbouring atoms. One can easily reproduce the MTC formula as $\kappa \approx 0.474(3/2 + D_v/2)k_B\bar{v}_s n_{\text{atom}}^{\frac{2}{3}}$ by choosing $D_v \approx 2$. We calculated the thermal conductivities of a-Si, a-Ge, a-$CdGeAs_2$, and v-$SiO_2$ with the parameters given in Table. S3. The calculated values are in good agreement with the measured ones as shown in Fig. 2(c) when $D_v$ is chosen to be 2.

### SC. Macromolecular chain segments as fundamental units in polymer solids and polymer liquids

Polymers solids and polymer melts consist of macromolecules with extremely long length, i. e. $L \gg a$. Therefore, it is inappropriate to consider an entire chain as one fundamental unit. It has been pointed out that there are three processes when a heat current flow through polymers [14, 15]: inter-chain heat transfer and intra-chain heat transfer at contact points and thermal transport inside each segment between two adjacent contact points. It is obvious that thermal equilibrium of each fundamental unit is faster than inter-chain heat transfer because of the large intrinsic thermal conductivity of a single molecular chain [16, 17]. Therefore, $\tilde{n} = \frac{L}{\xi}n_{\text{mole}}$, $\Xi = 4$ and $Z = 6$ as shown in Fig. 1(c). Zhou et al. [14] have evaluated that $\xi = 4\sqrt{\frac{m_{\text{unit}}}{l_{\text{unit}}\rho}}$ where $m_{\text{unit}}$ and $l_{\text{unit}}$ are the

TABLE S4. Mass density, length and molar mass of repeating unit, size of functional groups, and sound velocity of a-Se and six polymers: polypropylene (PP), Nylon 6, poly(ether ether ketone) (PEEK), Nylon-12, polystryrene (PS), and polytetrafluoroethylene (PTFE) [6, 14, 18, 19].

| Polymers | $\rho$ (g/cm$^3$) | $l_{\text{unit}}$ (Å) | $m_{\text{unit}} \times N_A$ (g/mol) | $a'$ (Å) | $v_{sl}$ (m/s) | $v_{st}$ (m/s) |
|---|---|---|---|---|---|---|
| PP | 0.85 | 2.17 | 42.1 | 4.0-7.1 | 3420 | 1750 |
| Nylon 6 | 0.65 | 8.6 | 113.2 | 4.0-5.6 | 3470 | 1610 |
| PEEK | 1.26 | 10 | 288.3 | 3.0-5.4 | 3000 | 1500 |
| Nylon 12 | 1.02 | 16 | 198 | 4.0-5.6 | 3380 | 1630 |
| PS | 1.05 | 3.32 | 104 | 4.0-8.4 | 2870 | 1480 |
| PTFE | 2.0 | 1.3 | 50.01 | 2.8-4.0 | 1350 | 550 |
| a-Se (polymer chain) | 4.3 | 1.88 | 78.96 | 3.80 | 2060 | 1060 |

mass and length of repeating units, respectively. Moreover, in isotropic polymers, $\frac{1}{h} = (1-\gamma)R_{\text{intra}} + \gamma R_{\text{inter}} \approx \frac{R_{\text{inter}}}{2}$ because $\gamma \approx (1-\gamma) \approx 1/2$ where $R_{\text{intra}}$ is the intra-chain thermal resistance which is negligible compared to $R_{\text{inter}}$ [14]. Therefore, the average value of $h$ can be obtained as $2\frac{C_{per}\bar{v}_s}{\delta}$. Eq. (1) is then reduced to Eq. (3) with $\alpha = \left(\frac{l_{\text{unit}}\rho}{m_{\text{unit}}}\right)^{1/2}$ as given in Fig. 1(c). It is easy to reproduce $\kappa_{\text{P}}$ by using $\frac{l_{\text{unit}}\rho}{m_{\text{unit}}} = \frac{L\rho}{M_{\text{mole}}} = Ln_{\text{mole}}$. The value of $\delta$ is determined by the size of functional groups, noted as $a'$, such as -$CH_3$, -F, -OH, =CO etc. We have performed molecular-dynamic (MD) simulation in Ref. [14] to clarify the impact of the intermolecular separation $\delta$ on the inter-chain thermal resistance. The MD simulations have demonstrated that the inter-chain thermal resistance severely depends on the intermolecular separation $\delta$. Here we evaluate the actual value of $\delta$ from van der Walls diameter of functional groups. This estimation is reasonable, while the accurate determination of $\delta$ deserves further investigation. Figure 2(d) shows the calculated thermal conductivity of several typical polymers in comparison with the experimental data, where $D_v = 1$ and other parameters are listed in Table. II.

### SD. Monte Carlo simulations

In order to evaluate the coordination number of molecules in liquid, the molecules are simplified into either spheres or cylinders with hemisphere at two ends, see Fig. S1. The positions of molecules are random, thus we adopted the Monte Carlo method to generate an equivalent liquid structure. We first evaluate the number $N_{\text{MC}}$ of particles generated in a given box, $N_{\text{MC}} = (\ell^3 \times \rho)/m_{\text{mole}}$. The size of the simulation box, $\ell$, is chosen to be 10 nm. Then the position of particles is randomly generated and recorded. Once a new particle is generated, the distance to the previously generated particles in the box will be calculated. If the distance is smaller than the van der Waals diameter given in Table. S1, it will be recorded as a contact point. After all particles has been generated, the total

contact number $N_{\text{contact}}$ is obtained. The average coordination number is then evaluated from $Z = 2 \times N_{\text{contact}}/N_{\text{MC}}$.

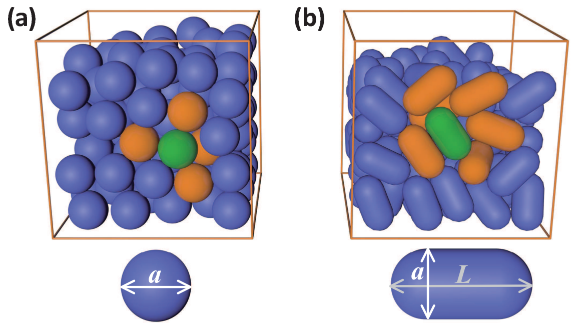


FIG. S1. (Color online) Random close packing of (a) spherical molecules and (b) capsule-like molecules which consists of a cylinder and two hemispherical ends. The diameter of sphere and the diameter of cylinder are noted as $a$. The length of capsule is $L$. Touching neighbours (in orange) of a certain molecule marked in green are shown.

* jliu38@ncsu.edu
† zhoujunzhou@tongji.edu.cn
‡ Baowen.Li@Colorado.edu

[1] K. Trachenko and V. V. Brazhkin, Sci. Rep. **3**, 2188 (2013).
[2] J. Frenkel, *Kinetic Theory of Liquids*, edt. R. H. Fowler, P. Kapitza, N. F. Mott, (Oxford University Press, 1947).
[3] J. C. Dyre, Rev. Mod. Phys. **78**, 953 (2006).
[4] P. G. De Gennes, *Scaling Concepts in Polymer Physics*, (Cornell University Press, New York, 1979).
[5] Extracted from https://pubchem.ncbi.nlm.nih.gov/.
[6] J. N. Israelachvii, *Intermolecular and Surface Forces*, (Academic Press, Boston, 2011), p134.
[7] T. Head-Gordon and M. E. Johnson, Proc. Natl. Acad. Sci. **21**, 7973 (2006).
[8] Z. H. Stachurski, *Fundamentals of Amorphous Solids: Structure and Properties*, (Higher Education Press, Beijing, 2015), p. 23, 116.
[9] D. G. Cahill, S. K. Watson, R. O. Pohl, Phys. Rev. B **46**, 6131 (1992).
[10] M. Kawarada and Y. Nishina, Jpn. J. Appl. Phys. **14**, 1519 (1975).
[11] B. E. Warren, J. Appl. Phys. **8**, 645 (1937); *ibid* **13**, 602 (1942).
[12] R. Zallen, *The Physics of Amorphous Solids*, (John Wiley & Sons, New York, 1998) p. 107-133.
[13] J. A. Barker, M. R. Hoare, and J. L. Finney, Nature **257**, 120 (1975).
[14] J. Zhou, Q. Xi, J. He, T. Nakayama, Y. Y. Wang, and J. Liu, Phys. Rev. Mater. **4**, 015601 (2020).
[15] L. Dong, Q. Xi, D. Chen, J. Guo, T. Nakayama, Y. Li, Z. Q. Liang, J. Zhou, X. F. Xu, and B. W. Li, Nat. Sci. Rev. **5**, 500 (2018).
[16] A. Henry and G. Chen, Phys. Rev. Lett. **101**, 235502 (2008).
[17] J. Liu and R. Yang, Phys. Rev. B **86**, 104307 (2012).
[18] J. E. Mark, *Polymer Data Handbook*, (Oxford University Press, Oxford, 2009).
[19] J. Robertson, Philos. Mag. **34**, 13 (1976).
